# Supplementary material for: Improving PINNs By Algebraic Inclusion of Boundary and Initial Conditions
Source: arXiv:2407.20741 source file (2024-07-30)
Supplement: Supplementary file 1 [file Standard_Appendix.tex]

\section{Some Notation}\label{sec:note} 

\note{ 
 
The following come from the ``physics'' package except the inner-product~\\ ~\\
$\ip{\va}{\vb}, \abs{c}, \norm{\vd}, \pdv{L}{\vw}, \pdv[2]{L}{\vw}, \dv{W}{t}, \dd{x}, \rank (\mM),\tr(\mA),\Tr (\mB), \var{W}$
~\\ ~\\ 
$\relu$ is our definition
~\\ 
We have also defined the following calligraphic letters, 
$\cF, \cR, \cN, \cE, \cL, \cD$
~\\
}

\begin{center} 
\hl{This is the default highlight!}
\om{This is our customized highlight!}
\end{center} 

\note{ Everything below comes from the TMLR format \\
- which comes from this book, \url{https://github.com/goodfeli/dlbook_notation/}}

\vspace{0.5cm} 
\centerline{\bf Sets and Graphs}
\bgroup

\begin{tabular}{p{1.25in}p{3.25in}}
$\sA$ & A set\\
$\R$ & The set of real numbers \\
$\{0, 1\}$ & The set containing 0 and 1 \\
$\{0, 1, \dots, n \}$ & The set of all integers between $0$ and $n$\\
$[a, b]$ & The real interval including $a$ and $b$\\
$(a, b]$ & The real interval excluding $a$ but including $b$\\
$\sA \backslash \sB$ & Set subtraction, i.e., the set containing the elements of $\sA$ that are not in $\sB$\\
$\gG$ & A graph\\
$\parents_\gG(\ervx_i)$ & The parents of $\ervx_i$ in $\gG$
\end{tabular}
\egroup 

~\\ ~\\
\centerline{\bf Numbers and Arrays}
\bgroup

\begin{tabular}{p{1in}p{3.25in}}
$a$ & A scalar (integer or real)\\
$\va$ & A vector\\
$\mA$ & A matrix\\
$\tA$ & A tensor\\
$\mI_n$ & Identity matrix with $n$ rows and $n$ columns\\
$\mI$ & Identity matrix with dimensionality implied by context\\
$\ve^{(i)}$ & Standard basis vector $[0,\dots,0,1,0,\dots,0]$ with a 1 at position $i$\\
$\text{diag}(\va)$ & A square, diagonal matrix with diagonal entries given by $\va$\\
$\ra$ & A scalar random variable\\
$\rva$ & A vector-valued random variable\\
$\rmA$ & A matrix-valued random variable\\
\end{tabular}
\egroup

~\\ ~\\ 
\centerline{\bf Indexing}
\bgroup

\begin{tabular}{p{1.25in}p{3.25in}}
$\eva_i$ & Element $i$ of vector $\va$, with indexing starting at 1 \\
$\eva_{-i}$ & All elements of vector $\va$ except for element $i$ \\
$\emA_{i,j}$ & Element $i, j$ of matrix $\mA$ \\
$\mA_{i, :}$ & Row $i$ of matrix $\mA$ \\
$\mA_{:, i}$ & Column $i$ of matrix $\mA$ \\
$\etA_{i, j, k}$ & Element $(i, j, k)$ of a 3-D tensor $\tA$\\
$\tA_{:, :, i}$ & 2-D slice of a 3-D tensor\\
$\erva_i$ & Element $i$ of the random vector $\rva$ \\
\end{tabular}
\egroup

~\\ ~\\ 
\centerline{\bf Probability and Information Theory}
\bgroup

\begin{tabular}{p{1.25in}p{3.25in}}
$P(\ra)$ & A probability distribution over a discrete variable\\
$p(\ra)$ & A probability distribution over a continuous variable, or over
a variable whose type has not been specified\\
$\ra \sim P$ & Random variable $\ra$ has distribution $P$\\% so thing on left of \sim should always be a random variable, with name beginning with \r
$\E_{\rx\sim P} [ f(x) ]\text{ or } \E f(x)$ & Expectation of $f(x)$ with respect to $P(\rx)$ \\
$\Var(f(x)) $ &  Variance of $f(x)$ under $P(\rx)$ \\
$\Cov(f(x),g(x)) $ & Covariance of $f(x)$ and $g(x)$ under $P(\rx)$\\
$H(\rx) $ & Shannon entropy of the random variable $\rx$\\
$\KL ( P \Vert Q ) $ & Kullback-Leibler divergence of P and Q \\
$\mathcal{N} ( \vx ; \vmu , \mSigma)$ & Gaussian distribution %
over $\vx$ with mean $\vmu$ and covariance $\mSigma$ \\
\end{tabular}
\egroup

~\\ ~\\ 
\centerline{\bf Functions}
\bgroup

\begin{tabular}{p{1.25in}p{3.25in}}
$ f: \sA \rightarrow \sB$ & The function $f$ with domain $\sA$ and range $\sB$\\
$ f \circ g $ & Composition of the functions $f$ and $g$ \\
$f(\vx ; \vtheta) $ & A function of $\vx$ parametrized by $\vtheta$.
  (Sometimes we write $f(\vx)$ and omit the argument $\vtheta$ to lighten notation) \\
$\log x$ & Natural logarithm of $x$ \\
$\sigma(x)$ & Logistic sigmoid, $\frac{1} {1 + \exp(-x)}$ \\
$\zeta(x)$ & Softplus, $\log(1 + \exp(x))$ \\
$\norm{\vx}_p $ & $L^p$ norm of $\vx$ \\
$\norm{\vx}$ & $L^2$ norm of $\vx$ \\
$x^+$ & Positive part of $x$, i.e., $\max(0,x)$\\
$\1_\mathrm{condition}$ & is 1 if the condition is true, 0 otherwise\\
$\argmax_{\rvx \in \R^n} f$\\  
$\argmin_{\rvx \in \R^n} f$\\
$\reg, \rect,\softmax,\sigmoid,\softplus,\Var,\standarderror$\\
\end{tabular}
\egroup

\clearpage 

\begin{theorem}\label{thm:jamini}
The world would be a better place if everyone read more about one of the greatest artists of this century, \href{https://artsandculture.google.com/story/jamini-roy-national-gallery-of-modern-art-ngma-new-delhi/OgWRKWgZqPzIJw?hl=en}{Jamini Roy}
\end{theorem}

\begin{proof}{(of Theorem \ref{thm:jamini})}
~\\ 
\begin{figure}[!h]
    \centering
    \includegraphics[width=\textwidth]{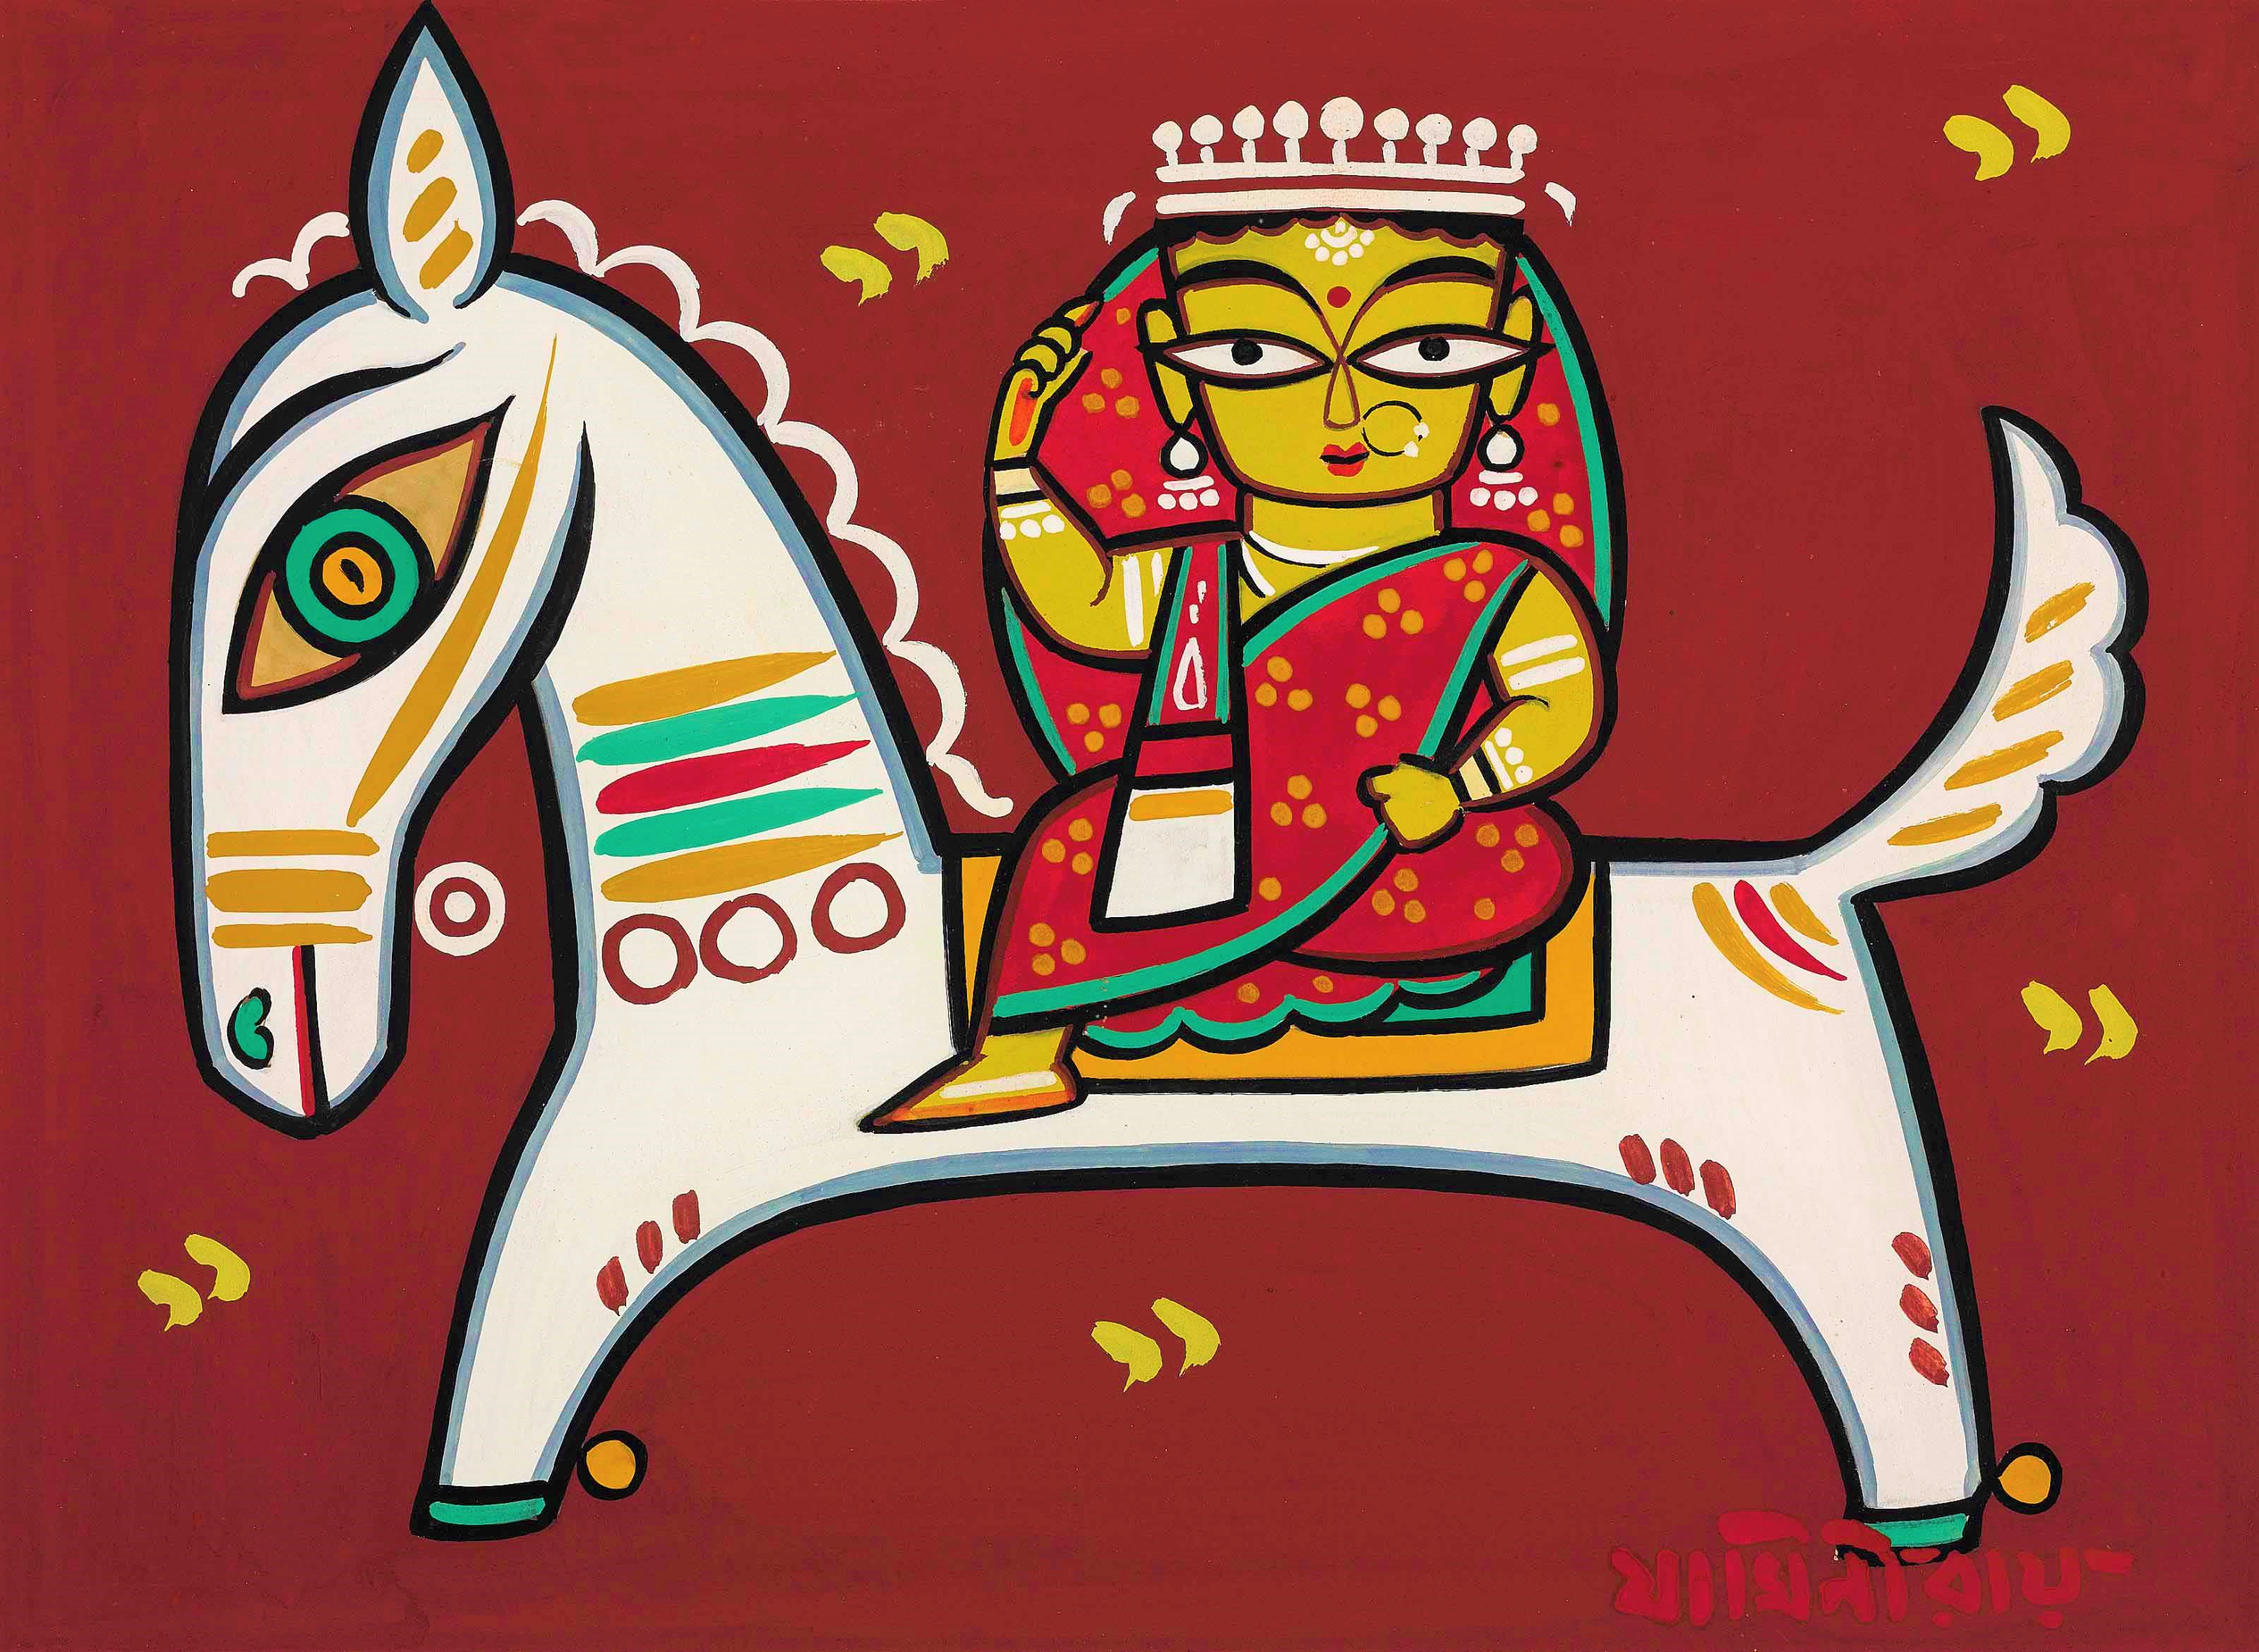}
    \caption{Hence Proved!}
    \label{fig:}
\end{figure}
\end{proof}

\begin{algorithm}[tb] 
\caption{Neuro-Tron (mini-batched, multi-gate, single-filter, stochastic algorithm)}
\label{minibatchneurotronsinglestoch}
\begin{algorithmic}[1]
\State {\bf Input:} Sampling access to the marginal input distribution ${\cal D}_{\rvx}$ % on $\R^n$
\State {\bf Input:} Access to adversarial output $\rvv\in\R$
for any input $\rvx\in\R^n$
 % adversarially corrupted output $y \in \R$ when queried with $\x \in \R^n$
 \State {\bf Input:} Access to output  $f_{\rvw} (\rvx)$ of any $f_\rvw \in  \mathcal{F}_{k,\alpha,\mathcal{A},{\cal W}}$
for any $\rvw\in \R^r$ and any input $\rvx$
\State {\bf Input:} A sensing matrix $\mM \in \R^{r \times n}$
\State {\bf Input:} A starting point $\vw_1$
\State {\bf Input:} Number $T$ of batches
\State {\bf Input:} Batch size $b$
\State {\bf Input:} Learning rate $\eta$
\For{$t = 1,\ldots$,\,{\rm T}}
    \State Sample batch
    $s_t \coloneqq
    (\rvx_{t_1},\ldots,\rvx_{t_b})$,
    where $\rvx_{t_i}\sim {\cal D}_{\rvx},~i=1,\ldots,b$ %and query the (adversarial) oracle with it.
    \For{$i = 1,\ldots,b$}
    \State  The oracle samples
    $\alpha_{t_i} \in \{0,1\}$ with probability
    $\{ 1 -\beta(\rvx_{t_i}), \beta(\rvx_{t_i})\}$
\State The oracle replies with
  $\rvv_{t_i} := f_{\vw^*}(\rvx_{t_i} )+\alpha_{t_i}\xi_{t_i}$
  \EndFor
  \State Form the so-called Tron-gradient, 
    \[\rvg^{(t)} := \mM \left ( \frac{1}{b} \sum_{i=1}^b
    \left ( \Big (\rvv_{t_i} - f_{\rvw^{(t)}}(\rvx_{t_i}) \Big) \rvx_{t_i} \right ) \right )\]
  \State  $\rvw^{(t+1)} = \rvw^{(t)} + \eta \rvg^{(t)}$
\EndFor 
\end{algorithmic}
\end{algorithm}

\clearpage 

\begin{equation}
\begin{aligned}[t]
x & =2+2\\
  & =3+1\\
  & =4
\end{aligned}
\end{equation}

\begin{equation}
\begin{aligned}[c]
y & =4+4\\
  & =7+1\\
  & =8
\end{aligned}
\end{equation} 

\begin{equation}
\begin{aligned}[b]
z & =6+6\\
  & =11+1\\
  & =12
\end{aligned}
\end{equation}
